# Supplementary material for: Quantum holography with undetected light
Source: arXiv:2106.04904 ancillary file (2022-04-29)
Supplement: Supplementary file 1 [file sm_Quantum_holography_with_undetected_light.pdf]

Supplementary Materials for

# Quantum holography with undetected light

Sebastian Töpfer, Marta Gilaberte Basset, Jorge Fuenzalida, Fabian Steinlechner, Juan P. Torres, and Markus Gräfe*

*Corresponding author. Email: markus.graefe@iof.fraunhofer.de

**This PDF file includes:**

Supplementary Text Figs. S1 to S5

# Theory of Phase-shifting holography with a SU(1,1) nonlinear interferometer

General equations

The experimental set-up is depicted in Fig. 2 of the main text. The bandwidth ($\Delta_{DC}$) of paired photons generated in parametric down-conversion (PDC) is much larger than the bandwidth of the pump beam ($\delta_p$). The Rayleigh length ($L_R = k_p^0 w_p^2/2$) of the pump beam is much larger than the crystal length ($L \gg L_R$). $w_p$ is the pump beam waist and $k_p^0 = 2\pi n_p/\lambda_p^0$ is the pump beam wavenumber. In this scenario we can describe the spatio-temporal characteristics of parametric down-conversion using the CW and plane pump beam approximation.

In the low parametric gain regime, the Bogoliuvov transformations that relate the quantum operators $a_s$ and $a_i$ at the output face of the nonlinear crystal to the quantum operators at the input face of the nonlinear crystal ($b_s$ and $b_i$) are [42, 43]

$$a_s(\mathbf{q}, \Omega) = U_s(\mathbf{q}, \Omega)\, b_s(\mathbf{q}, \Omega) + V_s(\mathbf{q}, \Omega)\, b_i^\dagger(-\mathbf{q}, -\Omega) \tag{S1}$$

$$a_i(\mathbf{q}, \Omega) = U_i(\mathbf{q}, \Omega)\, b_i(\mathbf{q}, \Omega) + V_i(\mathbf{q}, \Omega)\, b_s^\dagger(-\mathbf{q}, -\Omega) \tag{S2}$$

where

$$\begin{aligned} U_{s,i}(\mathbf{q}, \Omega) &= \exp\left[ik_{s,i}(\mathbf{q}, \Omega)L\right] \\ V_{s,i}(\mathbf{q}, \Omega) &= -i\,(\sigma L)\,\mathrm{sinc}\frac{\Delta_k L}{2}\exp\left\{i\left[k_p^0 + k_{s,i}(\mathbf{q}, \Omega) - k_{i,s}(-\mathbf{q}, -\Omega)\right]\frac{L}{2} + i\varphi_p\right\} \end{aligned} \tag{S3}$$

$\mathbf{q} = (q_x, q_y)$ designates the transverse wavenumber of signal/idler photons, $\Omega$ is the frequency deviation from the corresponding central frequency and $\varphi_p$ is the phase of the pump beam. The nonlinear coefficient $\sigma$ is

$$\sigma = \left(\frac{\hbar\omega_p\omega_s\omega_i[\chi^{(2)}]^2 F_0}{8\epsilon_0 c^3 S n_p n_s n_i}\right)^{1/2}. \tag{S4}$$

$F_0 = P_0/(\hbar\omega_p)$ is the flux rate density of pump photons (photons/s), $S$ is the area of the pump beam and $P_0$ is the pump power. The low parametric gain regime corresponds to a gain $G = \sigma L \ll 1$.

The signal and idler beams fulfill the paraxial approximation, so we can expand the corresponding wavenumbers in a Taylor series as $k_{s,i} = k_{s,i}^0 + D_s\Omega - |\mathbf{q}|^2/(2k_{s,i}^0)$. $D_{s,i}$

are inverse group velocities. We assume phase matching at the central frequencies, i.e., $k_p^0 = k_s^0 + k_i^0 \pm 2\pi/\Lambda$ where $\Lambda$ is the period of the poling of the nonlinear crystal. The phase matching function is thus

$$\Delta_k = D\Omega L - |\mathbf{q}|^2 \left[ \frac{1}{2k_s^0} + \frac{1}{2k_i^0} \right] \quad \text{(S5)}$$

with $D = D_s - D_i$. Under these conditions, the functions $U_{s,i}$ and $V_{s,i}$ are invariant under changes $q_{x,y} \Longrightarrow -q_{x,y}$, a feature that we will use later on to simplify the expressions obtained.

In the first pass by the nonlinear crystal signal ($s_1$) and idler ($i_1$) beams are generated (beam paths $b$ and $c$, respectively, in Fig. 2 of the main text). The corresponding quantum operators are $a_{s_1}(\mathbf{q}, \Omega)$ and $a_{i_1}(\mathbf{q}, \Omega)$. The signal beam traverses a 4f system with focal length $f$ with a mirror located in the middle of the imaging system. After traversing this system the signal beam is injected back into the nonlinear crystal. There might be losses $r_s$ in the signal path. The transformation of the quantum operator $a_{s_1}$ is

$$a_{s_1}(q_x, q_y, \Omega) \Longrightarrow r_s a_{s_1}(q_x, -q_y, \Omega) \exp(i\varphi_s) + f_s \quad \text{(S6)}$$

with $\varphi_s = 4k_s^0 f + \Delta\varphi$. $\Delta\varphi$ is a phase that introduces a phase difference between signal and idler beam paths and that will be important to perform Phase shifting digital holography. The operators $f_s$, that fulfill the commutation relationship $[f_s, f_s^\dagger] = [1 - |r_s|^2]$, take into account losses in the signal path [44]. Notice that the transformation $q_y \longrightarrow -q_y$ in Eq. (S6), that only affects the $y$ component of the wavenumber, is due to the peculiar 4f system that we are considering. It includes back-propagation caused by the presence of a mirror, which makes it different from other commonly considered 4f systems.

The idler beam $i_1$ traverses a 4f system with focal length $f$ with an object with transmission function $t(\mathbf{x}) = |t(\mathbf{x})| \exp[i\theta(\mathbf{x})]$ in the middle. The transformation of the quantum operator $a_{i_1}$ is

$$a_{i_1}(q_x, q_y, \Omega) \Longrightarrow t\left(\frac{\lambda_i f}{2\pi} q_x, -\frac{\lambda_i f}{2\pi} q_y\right) a_{i_1}(q_x, -q_y, \Omega) \exp(i\varphi_i) + f\left(\frac{\lambda_i f}{2\pi} q_x, -\frac{\lambda_i f}{2\pi} q_y\right) \quad \text{(S7)}$$

The phase is $\varphi_i = 4k_i^0 f$. The operators $f(\mathbf{q})$, that fulfill the commutation relationship

$$[f(\mathbf{q}), f^\dagger(\mathbf{q}')] = \left[1 - |t(\mathbf{q})|^2\right] \delta(\mathbf{q} - \mathbf{q}'), \quad \text{(S8)}$$

take into account the spatially-dependent losses induced by the transmission function.

The quantum operator that describes the signal beam $s_2$ is:

$$\begin{aligned}
&a_{s_2}(q_x,q_y,\Omega) = r_s U_{s_2}(\mathbf{q},\Omega) a_{s_1}(q_x,-q_y,\Omega)\exp(i\varphi_s) + U_{s_2}(\mathbf{q},\Omega) f_s \\
&+V_{s_2}(\mathbf{q},\Omega) t^*\left(-\frac{\lambda_i f}{2\pi}\,q_x, \frac{\lambda_i f}{2\pi}\,q_y\right) a_{i_1}^\dagger(-q_x,q_y,-\Omega)\exp(-i\varphi_i) \\
&+V_{s_2}(\mathbf{q},\Omega) f^\dagger\left(-\frac{\lambda_i f}{2\pi}\,q_x, \frac{\lambda_i f}{2\pi}\,q_y\right) \\
&= r_s U_{s_2}(\mathbf{q},\Omega)\left[U_{s_1}(\mathbf{q},\Omega) b_s(q_x,-q_y,\Omega) + V_{s_1}(\mathbf{q},\Omega) b_i^\dagger(-q_x,q_y,-\Omega)\right]\exp(i\varphi_s) \\
&+V_{s_2}(\mathbf{q},\Omega) t^*\left(-\frac{\lambda_i f}{2\pi}\,q_x, \frac{\lambda_i f}{2\pi}\,q_y\right) \\
&\times\left[U_{i_1}^*(\mathbf{q},-\Omega) b_i^\dagger(-q_x,q_y,-\Omega) + V_{i_1}^*(\mathbf{q},-\Omega) b_s(q_x,-q_y,\Omega)\right]\exp(-i\varphi_i) \\
&+V_{s_2}(\mathbf{q}) f^\dagger\left(-\frac{\lambda_i f}{2\pi}\,q_x, \frac{\lambda_i f}{2\pi}\,q_y\right) + U_{s_2}(\mathbf{q},\Omega) f_s \\
&= [r_s U_{s_2}(\mathbf{q},\Omega) U_{s_1}(\mathbf{q},\Omega)\exp(i\varphi_s) \\
&+V_{s_2}(\mathbf{q},\Omega) V_{i_1}^*(\mathbf{q},-\Omega) t^*\left(-\frac{\lambda_i f}{2\pi}\,q_x, \frac{\lambda_i f}{2\pi}\,q_y\right)\exp(-i\varphi_i)\Big]\, b_s(q_x,-q_y,\Omega) \\
&+ [r_s U_{s_2}(\mathbf{q},\Omega) V_{s_1}(\mathbf{q},\Omega)\exp(i\varphi_s) \\
&+U_{i_1}^*(\mathbf{q},-\Omega) V_{s_2}(\mathbf{q},\Omega) t^*\left(-\frac{\lambda_i f}{2\pi}\,q_x, \frac{\lambda_i f}{2\pi}\,q_y\right)\exp(-i\varphi_i)\Big]\, b_i^\dagger(-q_x,q_y,-\Omega) \\
&+V_{s_2}(\mathbf{q},\Omega) f^\dagger\left(-\frac{\lambda_i f}{2\pi}\,q_x, \frac{\lambda_i f}{2\pi}\,q_y\right) + U_{s_2}(\mathbf{q},\Omega) f_s\;. \qquad \text{(S9)}
\end{aligned}$$

<u>Spatial shape of the flux rate of signal photons $s_2$</u>

We measure the spatial distribution of the photon flux density corresponding to the signal beam $s_2$ with the help of a 2f system with focal length $f_d$. The flux rate of signal photons $s_2$ detected at time $t$ is

$$\langle N(\mathbf{x},t)\rangle = \int d\Omega_1 d\Omega_2 \exp\left[i(\Omega_1-\Omega_2)t\right]\left\langle a_{s_2}^\dagger\left(\frac{2\pi}{\lambda_s f_d}\mathbf{x},\Omega_1\right) a_{s_2}\left(\frac{2\pi}{\lambda_s f_d}\mathbf{x},\Omega_2\right)\right\rangle$$

After the 2f system we use an imaging system with magnification $M = -1$. We obtain

$$\langle N(\mathbf{x},t)\rangle = \left(\frac{2\pi}{\lambda_s f_d}\right)^2 \int d\Omega\, F(\Omega) \left|V_{s_1}\left(\frac{2\pi}{\lambda_s f_d}\mathbf{x},\Omega\right)\right|^2 \left\{1 - \left|\tau\left(-\frac{\lambda_i}{\lambda_s}\frac{f}{f_d}x, \frac{\lambda_i}{\lambda_s}\frac{f}{f_d}y\right)\right|^2 \right.$$
$$+ \left| r_s U_{s_2}\left(\frac{2\pi}{\lambda_s f_d}\mathbf{x},\Omega\right)\exp(i\varphi_s + i\varphi_{p_1}) \right.$$
$$\left.\left. + U_{i_1}^*\left(\frac{2\pi}{\lambda_s f_d}\mathbf{x},-\Omega\right)\tau^*\left(-\frac{\lambda_i}{\lambda_s}\frac{f}{f_d}x, \frac{\lambda_i}{\lambda_s}\frac{f}{f_d}y\right)\exp(-i\varphi_i + i\varphi_{p_2})\right|^2\right\}$$
$$= \left(\frac{2\pi}{\lambda_s f_d}\right)^2 \int d\Omega\, F(\Omega) \left|V_{s_2}\left(\frac{2\pi}{\lambda_s f_d}\mathbf{x},\Omega\right)\right|^2$$
$$\times \left\{1 + r_s^2 + r_s U_{s_2}\left(\frac{2\pi}{\lambda_s f_d}\mathbf{x},\Omega\right) U_{i_1}\left(\frac{2\pi}{\lambda_s f_d}\mathbf{x},-\Omega\right)\tau\left(-\frac{\lambda_i}{\lambda_s}\frac{f}{f_d}x, \frac{\lambda_i}{\lambda_s}\frac{f}{f_d}y\right)\right.$$
$$\times \exp(i\varphi_s + i\varphi_i + i\Delta\varphi_p) + r_s U_{s_2}^*\left(\frac{2\pi}{\lambda_s f_d}\mathbf{x},\Omega\right) U_{i_1}^*\left(\frac{2\pi}{\lambda_s f_d}\mathbf{x},-\Omega\right)$$
$$\left.\times \tau^*\left(-\frac{\lambda_i}{\lambda_s}\frac{f}{f_d}x, \frac{\lambda_i}{\lambda_s}\frac{f}{f_d}y\right)\exp(-i\varphi_s - i\varphi_i - i\Delta\varphi_p)\right\} \tag{S10}$$

where $\Delta\varphi_p = \varphi_{p_1} - \varphi_{p_2}$. $r_s$ designate losses in the signal path and we have included the effect of filtering by means of the function $F(\Omega)$. If we make use explicitly of the modulus and phase of the transmission coefficient $\tau(x,y) = |\tau(x,y)|\exp[i\theta(x,y)]$, we have

$$\langle N(\mathbf{x},t)\rangle = \left(\frac{2\pi}{\lambda_s f_d}\right)^2 \int d\Omega\, F(\Omega) \left|V_{s_1}\left(\frac{2\pi}{\lambda_s f_d}\mathbf{x},\Omega\right)\right|^2 \left\{1 + r_s^2 + 2r_s\left|\tau\left(-\frac{\lambda_i}{\lambda_s}\frac{f}{f_d}x, \frac{\lambda_i}{\lambda_s}\frac{f}{f_d}y\right)\right|\right.$$
$$\left.\times \cos\left[\varphi_0 + D\Omega L - \left(\frac{2\pi}{\lambda_s f_d}\right)^2 L\left(\frac{1}{2k_s^0} + \frac{1}{2k_i^0}\right)|\mathbf{x}|^2 + \theta\left(-\frac{\lambda_i}{\lambda_s}\frac{f}{f_d}x, \frac{\lambda_i}{\lambda_s}\frac{f}{f_d}y\right)\right]\right\} \tag{S11}$$

where $\varphi_0 = \varphi_s + \varphi_i + \Delta\varphi_p + k_s^0 L + k_i^0 L$ is a constant phase.

## Amplitude and phase retrieval with phase shifting holography

We consider the measurement of $\langle N(\mathbf{x},t)\rangle$ for four values of the reference phase, $\varphi_0 = 0, \pi/2, \pi, 3\pi/2$. Let us designate

$$\nu = \left(\frac{2\pi}{\lambda_s f_d}\right)^2 L\left(\frac{1}{2k_s^0} + \frac{1}{2k_i^0}\right) = \frac{\pi L}{(\lambda_s f_d)^2}\left(\frac{\lambda_s}{n_s} + \frac{\lambda_i}{n_i}\right) \tag{S12}$$

and $r_0 = 1 + r_s^2$. We can write

$$N_0(\mathbf{x}) = \alpha \int d\Omega F(\Omega) \left| V_{s_1}\left(\frac{2\pi}{\lambda_s f}\mathbf{x}, \Omega\right)\right|^2 \times \left\{ r_0 + 2r_s \left|\tau\left(-\frac{\lambda_i}{\lambda_s}\frac{f}{f_d}x, \frac{\lambda_i}{\lambda_s}\frac{f}{f_d}y\right)\right| \cos\left[\theta\left(-\frac{\lambda_i}{\lambda_s}\frac{f}{f_d}x, \frac{\lambda_i}{\lambda_s}\frac{f}{f_d}y\right) + D\Omega L - \nu|\mathbf{x}|^2\right]\right\} \tag{S13}$$

$$N_{\pi/2}(\mathbf{x}) = \alpha \int d\Omega F(\Omega) \left| V_{s_1}\left(\frac{2\pi}{\lambda_s f}\mathbf{x}, \Omega\right)\right|^2 \times \left\{ r_0 - 2r_s \left|\tau\left(-\frac{\lambda_i}{\lambda_s}\frac{f}{f_d}x, \frac{\lambda_i}{\lambda_s}\frac{f}{f_d}y\right)\right| \sin\left[\theta\left(-\frac{\lambda_i}{\lambda_s}\frac{f}{f_d}x, \frac{\lambda_i}{\lambda_s}\frac{f}{f_d}y\right) + D\Omega L - \nu|\mathbf{x}|^2\right]\right\} \tag{S14}$$

$$N_{\pi}(\mathbf{x}) = \alpha \int d\Omega F(\Omega) \left| V_{s_1}\left(\frac{2\pi}{\lambda_s f}\mathbf{x}, \Omega\right)\right|^2 \times \left\{ r_0 - 2r_s \left|\tau\left(-\frac{\lambda_i}{\lambda_s}\frac{f}{f_d}x, \frac{\lambda_i}{\lambda_s}\frac{f}{f_d}y\right)\right| \cos\left[\theta\left(-\frac{\lambda_i}{\lambda_s}\frac{f}{f_d}x, \frac{\lambda_i}{\lambda_s}\frac{f}{f_d}y\right) + D\Omega L - \nu|\mathbf{x}|^2\right]\right\} \tag{S15}$$

$$N_{3\pi/2}(\mathbf{x}) = \alpha \int d\Omega F(\Omega) \left| V_{s_1}\left(\frac{2\pi}{\lambda_s f}\mathbf{x}, \Omega\right)\right|^2 \times \left\{ r_0 + 2r_s \left|\tau\left(-\frac{\lambda_i}{\lambda_s}\frac{f}{f_d}x, \frac{\lambda_i}{\lambda_s}\frac{f}{f_d}y\right)\right| \sin\left[\theta\left(-\frac{\lambda_i}{\lambda_s}\frac{f}{f_d}x, \frac{\lambda_i}{\lambda_s}\frac{f}{f_d}y\right) + D\Omega L - \nu|\mathbf{x}|^2\right]\right\} \tag{S16}$$

where $\alpha$ is a constant that depends on the detection efficiency and $F(\Omega)$ describes the frequency response of a frequency filter.

The phase of the transmission function can be evaluated with

$$\theta\left(-\frac{\lambda_i}{\lambda_s}\frac{f}{f_d}x, \frac{\lambda_i}{\lambda_s}\frac{f}{f_d}y\right) = \tan^{-1}\frac{N_{3\pi/2}(\mathbf{x}) - N_{\pi/2}(\mathbf{x})}{N_0(\mathbf{x}) - N_{\pi}(\mathbf{x})} + \nu|\mathbf{x}|^2 \tag{S17}$$

We can get rid of the phase induced by the parametric process, i.e. $\nu|\mathbf{x}|^2$, by subtracting the phases calculated with and without object present.

The amplitude can be evaluated by

$$\left|\tau\left(-\frac{\lambda_i}{\lambda_s}\frac{f}{f_d}x, \frac{\lambda_i}{\lambda_s}\frac{f}{f_d}y\right)\right| = \frac{1+r_s^2}{r_s}\,\frac{\left\{[N_0(\mathbf{x}) - N_{\pi}(\mathbf{x})]^2 + \left[N_{\pi/2}(\mathbf{x}) - N_{3\pi/2}(\mathbf{x})\right]^2\right\}^{1/2}}{N_0(\mathbf{x}) + N_{\pi/2}(\mathbf{x}) + N_{\pi}(\mathbf{x}) + N_{3\pi/2}(\mathbf{x})} \tag{S18}$$

We are not considering that pixels have a finite size $S$ centered around the center position $\mathbf{x}_0$ of each pixel. We can take into account this effect making the substitutions $N_{\Delta\varphi}(\mathbf{x}_0) \implies \int_S d\mathbf{x} N_{\Delta\varphi}(\mathbf{x})$. As a result images of sharp edges will be seen as smoother transitions.

Effect of the bandwidth of PDC in amplitude and phase retrieval: analytical approximation

To help understanding the effect of the bandwidth of PDC in phase shifting holography, we notice that Eqs. (S14), (S15), (S16) and (S17) can be well approximated as

$$I = r_0 \int d\Omega \exp\left[-\frac{\Omega^2}{B_f^2} - \gamma^2\left(\frac{D\Omega L}{2} - \frac{\nu|\mathbf{x}|^2}{2}\right)^2\right]$$
$$+2r_s|t| \int d\Omega \exp\left[-\frac{\Omega^2}{B_f^2} - \gamma^2\left(\frac{D\Omega L}{2} - \frac{\nu|\mathbf{x}|^2}{2}\right)^2\right] \cos\left[D\Omega L + \varphi_0 - \nu|\mathbf{x}|^2 + \theta\right] \quad \text{(S19)}$$

We have assumed Gaussian filtering $F(\Omega) = \exp(-\Omega^2/B_f^2)$ and we have approximated the sinc function by an exponential: $\text{sinc}^2\, x \sim \exp(-\gamma^2 x^2)$ with the same FWHM ($\gamma^2 = 0.3588$). The bandwidth of PDC is $B_{dc} = 4/[\gamma^2(DL)^2]$.

These integrals have analytical expressions and yield

$$I = \left(\frac{4\pi B_f^2}{4+\gamma^2(DL)^2B_f^2}\right)^{1/2} \exp\left\{-\frac{\gamma^2\nu^2|\mathbf{x}|^4}{4} + \frac{4B_f^2}{4+\gamma^2(DL)^2B_f^2}\frac{\gamma^4(DL)^2\nu^2|\mathbf{x}|^4}{16}\right\} \quad \text{(S20)}$$
$$+\left\{r_0 + 2r_s|t| \exp\left(-\frac{B_f^2(DL)^2}{4+\gamma^2(DL)^2B_f^2}\right)\cos\left[\varphi_0 + \theta - \nu|\mathbf{x}|^2\left(1 - \frac{\gamma^2(DL)^2B_f^2}{4+\gamma^2(DL)^2B_f^2}\right)\right]\right\}$$

Two main conclusions can be drawn from Eq. (S20). The first conclusion is that the bandwidth of PDC makes that the amplitude measured with phase shifting holography is not the real amplitude of the object ($|t|$) but an effective value $|t|_{eff} = |t| \exp\left(-\frac{B_f^2(DL)^2}{4+\gamma^2(DL)^2B_f^2}\right)$. For small bandwidths ($B_f \longrightarrow 0$) the correct amplitude $|t|$ is retrieved However, for larger bandwidth $|t|_{eff} \exp\left(-\frac{1}{\gamma^2}\right)$. Taking into account that

$$\int d\Omega \, \exp\left(-\frac{\gamma^2(DL)^2\Omega^2}{4}\right)[1+\cos(D\Omega L+\theta)] = \frac{\sqrt{4\pi}}{\gamma(DL)}\left[1+\exp\left(-\frac{1}{\gamma^2}\right)\cos\theta\right] \quad \text{(S21)}$$

we notice that the factor $\exp(-1/\gamma^2) = 0.06$ is the loss of visibility that one would observe in an interference experiment due to the finite bandwidth of the signal. We should highlight that using the exact solution with the sinc function we would have obtained 0.

The second conclusion is that the phase induced by the PDC process is modified, i.e., $\nu|\mathbf{x}|^2 \Longrightarrow \nu|\mathbf{x}|^2\left[1 - \left(\gamma^2(DL)^2B_f^2\right)/\left(4+\gamma^2(DL)^2B_f^2\right)\right]$. However when subtracting phases measured with and without the object, the phase of the object $\theta$ can still be correctly retrieved even for large bandwidths.

## Influence of the spatial resolution on the interference amplitude

The modulation images shown in this paper have a visible modulation drop on places where a step-like phase change is located (see Fig. S1). This behaviour is caused by the limited spatial resolution. The interference patterns overlap partially in this areas, resulting in sum to a new interference with lower amplitude. Figure S2 shows this behaviour simulated with two interference patterns of the same base amplitude and phase-steps of the same value as our samples. The phase-step with limited resolution was simulated by shaping the base amplitudes as error-functions. The graph shows that we can expect amplitude drops to 28% for a $0.82\pi$ phase-step and 56% for a $0.62\pi$ phase-step in the ideal case. In the case of $0.82\pi$ we could measure a drop to 38% of the amplitude. The difference may be caused by measurement imperfections.

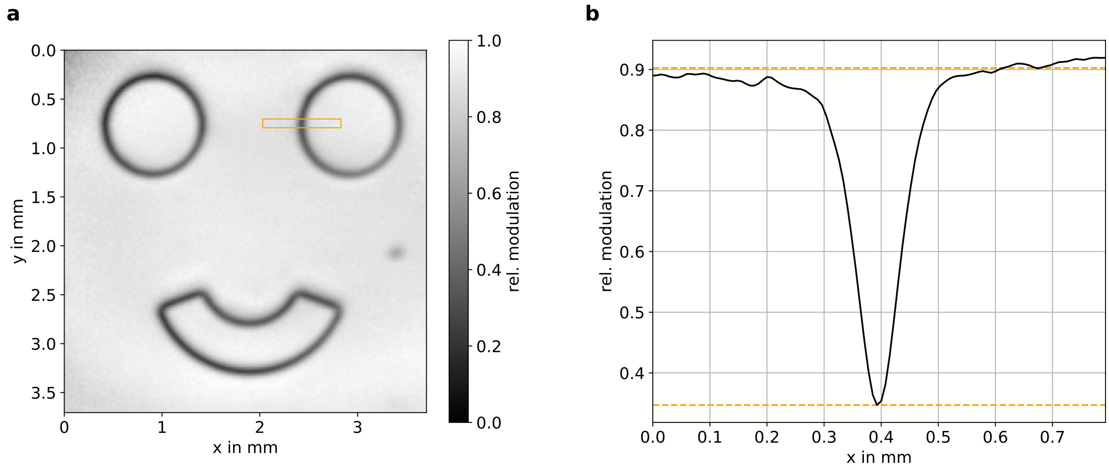


Figure S1: **Modulation drop profile.**(a) Modulation image of the happy face target with a phase-step of $0.82\pi$. (b) Profile of the modulation in the marked are with visible drop due to interference amplitude decrease.

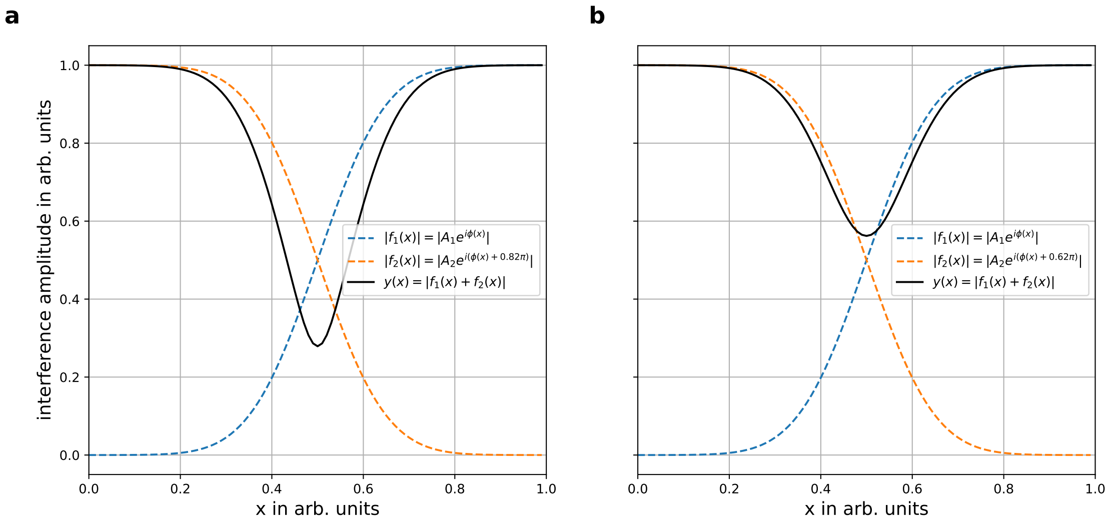


Figure S2: **Simulated interference amplitude drop**. The interference amplitude drops due to overlapping interference patterns, caused by limited spatial resolution for (a) $0.82\pi$ and (b) $0.62\pi$ phase difference.

## Object dimensions

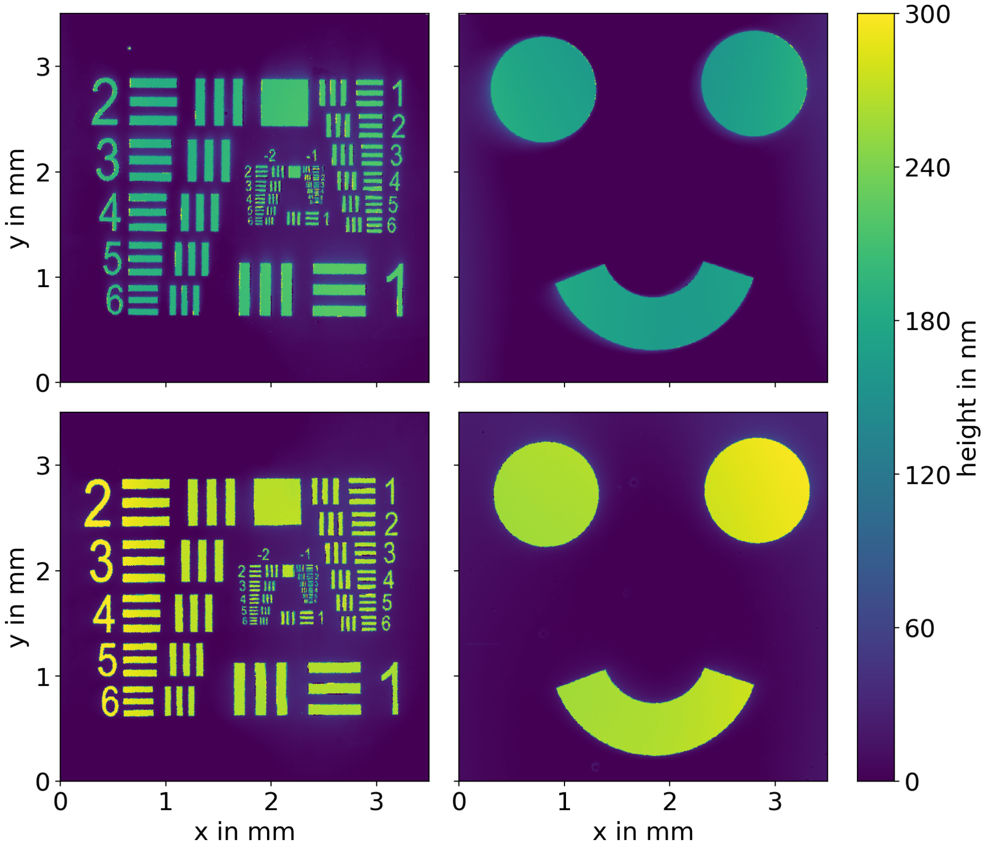


Figure S3: **Dimensions of the sample objects.** (top row) Miniaturized USAF and smiley phase targets manufactured to introduce a $0.62\pi$ phase shift. (bottom row) Miniaturized USAF and smiley phase targets manufactured to introduce a $0.82\pi$ phase shift. The phase shift introduced is calculated from the path difference seen for light at 730 nm travelling through the different sample thickness (height colorbar).

## Measured phase and transmission noise

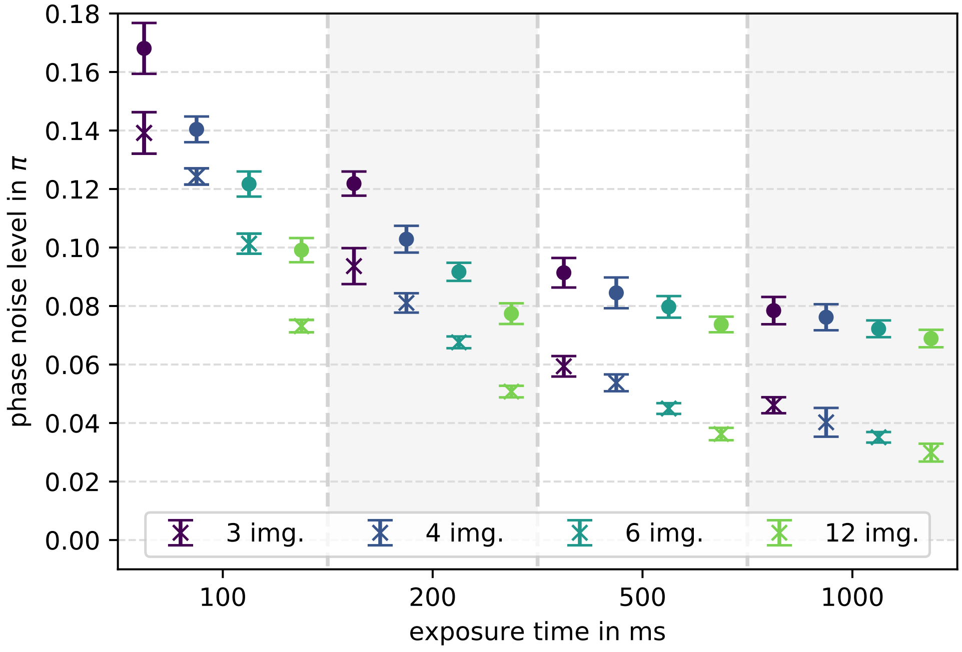


Figure S4: **Measured phase noise level.** The noise is measured as the standard deviation of the phase values at the high level of the phase step. Each points is an average of 15 image sets. The color is in relation to the amount of image used for the calculation of one phase image (see legend). The cross markers refer to a sample with a step size of $0.62\pi$ and the bullet markers refer to a sample with $0.82\pi$ step.

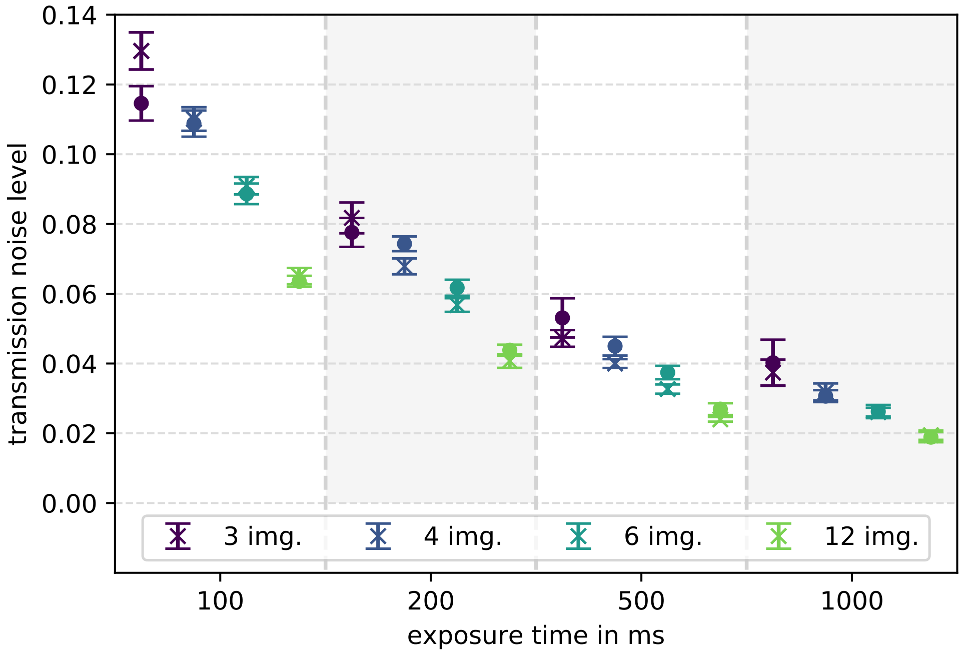


Figure S5: **Measured transmission noise level.** The noise is measured as the standard deviation of the transmission values. Each points is an average of 15 image sets. The color is in relation to the amount of image used for the calculation of one modulation image (see legend). The cross markers refer to a sample with a step size of $0.62\pi$ and the bullet markers refer to a sample with $0.82\pi$ step.
